# Supplementary material for: One2Any: One-Reference 6D Pose Estimation for Any Object
Source: arXiv:2505.04109 source file (2025-05-07)
Supplement: Supplementary file 1 [file 1_training_details.tex]

\section{Training Details}
\label{sec:training_details}
We describe the training process of our model, including the preprocessing of the data, and the network architecture details.
% which builds on the strengths of pre-trained architectures while incorporating specific modifications to generate ROC maps optimized for pose prediction tasks. To enhance training efficiency and address the unique characteristics of ROC maps compared to standard RGB images, the decoder is trained from scratch. The resulting OPD module efficiently generates ROC maps aligned with the reference coordinate system, enabling robust object pose estimation across diverse viewpoints. Throughout both the main text and the supplementary material, ROC maps are represented by their final output point clouds,  $Y_Q$  or  $Y_A$ , despite being parametrized by image pixel locations.

\subsection{Preprocessing of the Data }
We begin by masking each object in the image, cropping it so the object is centered, and resizing it to a resolution of  $192\times 192$. 

\noindent{}\textbf{Scale matrix $\mathbf{S}$. } The scale matrix $\mathbf{S}$ is obtained from the reference image $A$. The computation of the scale matrix $\mathbf{S}$  is detailed here. Let  $d^{A_D}$ represent the depth values in $A_D$, and $\begin{bmatrix} u \\ v \end{bmatrix} ^{A_D}$ denote the corresponding pixel positions of the object, pre-filtered using the mask $A_M$. The corresponding 3D point in the camera coordinate space for each pixel in the image  A  is given as $\begin{bmatrix} x \\ y \\ z \end{bmatrix} \in \mathbb{R}^3$.  Using this, we construct a point cloud$P_A \in \mathbb{R}^{N\times 3}$  where  $N$  is the number of points, computed as $N = \sum_{u}\sum_{v}{Q_M(u,v)=1}$.

To normalize the points into ROC space,  we apply the scale matrix $\mathbf{S}$, as defined in Equation \ref{eq:scale}. For each instance in the reference image, we establish a Reference Object Coordinate (ROC).

\begin{align}
\label{eq:scale}
        w = \operatorname{max}(\operatorname{max}(\begin{bmatrix} x \\ y \\z \end{bmatrix}^{P_A}) &- \operatorname{min}(\begin{bmatrix} x \\ y \\z \end{bmatrix}^{P_A}))\\
    c = \begin{bmatrix} c_x \\ c_y \\c_z \end{bmatrix}^{P_A} = (\operatorname{max}(\begin{bmatrix} x \\ y \\z \end{bmatrix}^{P_A})& + \operatorname{min}(\begin{bmatrix} x \\ y \\z \end{bmatrix}^{P_A})) / 2 \\
     Y_A = (Y_A - c) &/ (w \times 1.1) 
     % {p_A}^{\mathbb{O}} & += 0.5\\
    \end{align}
By determining the size scalar $w$ and the center $c$ of the point cloud $P_A$, we translate $P_A$ to the origin with the offset $c$ and scale it with $w \times 1.1$ to ensure all points lie within $[-0.5, 0.5]$. The result is the normalized 3D point cloud ${P_A}$ in ROC space, which is then mapped into an RGB image $Y_A$, referred to as the ROC map, where the RGB channels encode the 3D ROC positions.
%In detail, we find the maximum size $w^{P_A}$ and the center $c^{P_A}$ of the point cloud $P_A$, and we just move $P_A$ to the origin in the camera coordinate and scale it with $ 1 / (w^{P_A} \times 1.1)$ to make sure all points are within [-0.5, 0.5], and in the end move to [0,1] space.

In this process, the scale and shift transformation matrix $\mathbf{S}$ is also computed and recorded for further alignment on the predicted ROC map from the test image.
\begin{align}
     s &= 1 / (w \times 1.1) \\
     t &=  -1 \times c / s\\
     \mathbf{S} &= 
        {\begin{bmatrix}
     s & 0 & 0  & t_x\\
    0 &  s & 0 &t_y\\
   0 & 0 &  s & t_z \\
   0 & 0 & 0 & 1\\
\end{bmatrix}}
\end{align}

\subsection{Network Architecture}
\textbf{Diffusion Model \cite{rombach2022high}. } The text-to-image diffusion model is a generative framework designed to create high-quality images from textual descriptions. Its architecture consists of three key modules: an encoder and a decoder, based on VQVAE \cite{esser2021taming}, which map features between the image and latent spaces, and a U-Net module that performs denoising within the latent space. The diffusion proves its strong capability in image generation, and it can also cooperate with other generation tasks like depth generation \cite{ke2024repurposing}. Here, we extend the diffusion model to predict ROC maps. To improve time efficiency, we employ a feedforward stable diffusion model instead of the traditional iterative denoising process.

Following \cite{cai2024ov9d}, we utilize the stable diffusion model \cite{rombach2022high}, pre-trained on Laion-5b \cite{schuhmann2022laion}. We freeze the VQVAE module to encode the input query image $Q_{I}$, mapping it to the latent space as the feature map $\mathcal{F}^Q$. The U-Net is fine-tuned using our data pairs. Reference RGBD images serve as conditional inputs, processed through the Reference Object Encoder (ROE) and passed into the U-Net as feature maps  $\mathcal{F}^{A}$. The two feature embeddings $\mathcal{F}^Q$ and $\mathcal{F}^A$ , are integrated via the cross-attention modules in U-Net, producing the semantic and spatially aligned feature map $\mathcal{F}^{Q2A}$.  Since ROC maps differ significantly from typical RGB images, we train the decoder from scratch. The decoder progressively refines $\mathcal{F}^{Q2A}$  to reconstruct a high-resolution output aligned with the original image dimensions. The individual modules are detailed below.

\noindent{}\textbf{VQVAE. } We adopt the pre-trained VQVAE module from \cite{rombach2022high} and freeze it during training. Input images are normalized for better feature extraction.

\noindent{}\textbf{U-Net. } The U-Net is initialized with pre-trained weights from \cite{rombach2022high}. During the feedforward pass, no noise is added, allowing the U-Net to directly output meaningful feature embeddings. The ROE features serve as conditional inputs to the U-Net, interacting with the latent feature $\mathcal{F}^{Q}$ through cross-attention layers. The U-Net gradually learns to process the feature maps from ROPE and the test image.

\noindent{}\textbf{ROE.} The Reference Object Encoder (ROE), denoted as  $f(A; \theta_A)$  extracts latent encodings from a channel-wise concatenation of the reference RGB image, ROC map, and object mask. This encoding captures both texture and geometric information. The ROE processes these inputs through three convolutional layers with batch normalization and ReLU activation. A residual connection block \cite{he2016deep} further refines the features embeddings. The resulting feature maps are tokenized into patches with positional embeddings \cite{alexey2020image}, effectively guiding ROC map generation and maintaining fidelity to reference data, even under occlusion.

\noindent{}\textbf{Decoder.} The decoder consists of five convolutional layers with residual connections \cite{he2016deep}. Each layer includes a bilinear upsampling module to produce the final ROC map  $\hat{Y}_{Q}$. The decoder is initialized using Kaiming Initialization \cite{he2015delving}.
