# Supplementary material for: One2Any: One-Reference 6D Pose Estimation for Any Object
Source: arXiv:2505.04109 source file (2025-05-07)
Supplement: Supplementary file 2 [file 2_more_experimental_results.tex]

\section{Experimental Results}
\label{sec:experimental_results}
In this section, we provide a detailed analysis of the experimental results and investigate the impact of training data scale on the performance of our model.

\subsection{Full Test Results on the YCB-Video Dataset}
We present the detailed test results on the YCB-Video \cite{xiang2017posecnn} test set in Table \ref{tab:ycbv_data_full}, including performance metrics for each object. For all one-view methods, only the first test image is used as the reference image. In contrast, multi-view-based methods such as FS6D \cite{he2022fs6d}, Predator \cite{huang2021predator}, and LoFTR \cite{sun2021loftr} are fine-tuned on the test set, following the protocol outlined in FS6D \cite{he2022fs6d}. Specifically, FS6D divides the test objects into three groups, training on two groups while testing on the remaining one. Our method demonstrates superior performance compared to other one-view-based approaches, particularly for the ADD metric, where it significantly outperforms all competing methods. Our method even surpasses some multi-view approaches that employ fine-tuning on the test data.

\begin{table*}[]
    \centering
    \footnotesize
       \setlength{\tabcolsep}{0.2mm}
    \caption{Performance on occluded YCB-Video \cite{xiang2017posecnn} dataset. We compare with point cloud registration methods, multi-view methods, and one-view methods. Predator \cite{huang2021predator}, LoFTR \cite{sun2021loftr} and FS6D \cite{he2022fs6d} are fine-tuned on the YCB-Video dataset. We evaluate ADD-S AUC and ADD AUC metrics. Results of multi-view methods are adopted from \cite{wen2024foundationpose}. For one-view methods, we provide the first image in the test set as the reference. The best performance among multi-view methods and one-view methods are highlighted in bold.}
    % \vspace{-0.3cm}
    \begin{tabular}{c| c c | c c |c c |c c || c c | c c | c c | c c}
    \toprule
        Methods  &\multicolumn{2}{c|}{\textbf{PREDATOR} \cite{huang2021predator}} & \multicolumn{2}{c|}{\textbf{LoFTR}\cite{sun2021loftr}} &  \multicolumn{2}{c|}{\textbf{FS6D} \cite{he2022fs6d}} & \multicolumn{2}{c||}{\textbf{FoundationPose} \cite{wen2024foundationpose}} &  \multicolumn{2}{c|}{\textbf{FoundationPose}\cite{wen2024foundationpose}} &  \multicolumn{2}{c|}{\textbf{Oryon} \cite{corsetti2024open}} &  \multicolumn{2}{c|}{\textbf{NOPE} \cite{nguyen2024nope}} & \multicolumn{2}{c}{\textbf{One2Any(Ours)}} \\
  
        Ref. Images & \multicolumn{2}{c|}{16} & \multicolumn{2}{c|}{16} & \multicolumn{2}{c|}{16} & \multicolumn{2}{c|}{16 - CAD}  & \multicolumn{2}{c|}{1 - CAD} & \multicolumn{2}{c|}{1} & \multicolumn{2}{c|}{1 + GT trans} & \multicolumn{2}{c}{1} \\
        \midrule
        metrics & ADD-S & ADD & ADD-S & ADD  & ADD-S & ADD  & ADD-S & ADD & ADD-S & ADD & ADD-S & ADD & ADD-S & ADD & ADD-S & ADD \\
        \midrule
       002\_master\_chef\_can  &73.0 & 17.4 & 87.2 & 50.6& 92.6 & 36.8 & \textbf{96.9} & \textbf{91.3} &87.3 & 73.3 &  12.2 & 8.7 & 96.8 & 17.8 & \textbf{94.9} & \textbf{84.3}\\
003\_cracker\_box & 41.7 & 8.3 & 71.8 & 25.5  & 83.9 & 24.5 & \textbf{97.5} & \textbf{96.2} & \textbf{92.0}	& 72.2 &  6.5 & 3.3 & 83.0 & 2.8 & 91.1 & \textbf{83.3}\\
004\_sugar\_box &  53.7 & 15.3 & 63.9 & 13.4 & 95.1 & 43.9 & \textbf{97.5} & \textbf{87.2} &  88.2	&87.1 &  5.3 & 3.8 & 86.5 & 22.3 & \textbf{95.3} &\textbf{88.0} \\
005\_tomato\_soup\_can & 81.2 & 44.4 & 77.1 & 52.9 & 93.0 & 54.2 & \textbf{97.6} & \textbf{93.3} & 95.2 &	\textbf{92.3} & 10.9 & 5.9  & \textbf{95.9} & 48.4  & 93.6 & 80.9 \\
006\_mustard\_bottle &  35.5 & 5.0 & 84.5 & 59.0&  97.0 & 71.1 & \textbf{98.4} & \textbf{97.3} & 88.4 &	76.6 &  5.5 & 4.7 & 91.3 & 42.7 & \textbf{93.8} & \textbf{87.6}\\
007\_tuna\_fish\_can &  78.2 & 34.2 & 72.6 & 55.7 & 94.5 & 53.9 & \textbf{97.7} & \textbf{73.7} & 90.5 &	76.9 &23.2 & 15.6 &\textbf{97.0} & 33.3 & \textbf{95.9} & \textbf{90.0}\\
008\_pudding\_box &  73.5 & 24.2 & 86.5 & 68.1& 94.9 & 79.6 & \textbf{98.5} & \textbf{97.0} & 91.7 &	77.8 & 1.3 & 1.3 & 84.4 & 20.9 & \textbf{96.1} & \textbf{93.3} \\
009\_gelatin\_box &  81.4 & 37.5 & 71.6 & 45.2 & 98.3 & 32.1 & \textbf{98.5} & \textbf{97.3} & 92.7& 87.7 & 1.3 & 1.3 & 87.3 & 35.3 & \textbf{97.7} & \textbf{96.1}\\
010\_potted\_meat\_can &  62.0 & 20.9 & 67.4 & 45.1 & 87.6 & 54.9 & \textbf{96.6} & \textbf{82.3} & 90.3 & \textbf{83.5} & 38.9 & 19.2 & \textbf{92.8} & 31.9 & 86.3 &  72.5\\
011\_banana &  57.7 & 9.9 & 24.2 & 1.6 & 94.0 & 69.1 & \textbf{98.1} & \textbf{95.4} &90.3	& 76.3 & 4.9 & 4.1 & 61.3 & 11.4 & \textbf{95.0} & \textbf{85.7}\\
019\_pitcher\_base &  83.7 & 18.1 & 58.7 & 22.3 & 91.1 & 40.4 & \textbf{97.9} & \textbf{96.6} & 92.1 &	86.9 & 41.2 & 14.9 & 88.9 & 6.1 & \textbf{93.6} & \textbf{87.7}\\
021\_bleach\_cleanser & 88.3 & 48.1 & 36.9 & 16.7 & 89.4 & 44.1 & \textbf{97.4} & \textbf{93.3} & 90.8	& \textbf{85.5} &  5.0 & 2.8 & 89.6 & 32.3 & \textbf{93.0} & 84.6 \\
024\_bowl & 73.2 & 17.4 & 32.7 & 1.4 & 74.7 & 0.9 & \textbf{94.9} & \textbf{89.7} & 87.5	& 43.6 & 3.8 & 3.6 & \textbf{93.2} & 6.7 & 92.1 & \textbf{65.1}\\
025\_mug &  84.8 & 29.5 & 47.3 & 23.6& 86.5 & 39.2 & \textbf{96.2} & \textbf{75.8} &91.0 &	74.1 & 2.6 & 2.6 & 92.5 & 31.6 & \textbf{95.5} &  \textbf{82.9} \\
035\_power\_drill & 60.6 & 12.3 & 18.8 & 1.3 & 73.0 & 19.8 & \textbf{98.0} & \textbf{96.3} & \textbf{97.0}	& \textbf{96.8} &  22.1 & 13.1 & 56.0 & 0.0 & 92.4 & 84.6\\
036\_wood\_block &  70.5 & 10.0 & 49.9 & 1.4 & 94.7 & 27.9 & \textbf{97.4} & \textbf{94.7} & 67.1 &	19.9& 26.3 & 10.5 & 77.1 & 0.0 & \textbf{92.7} & \textbf{85.0}\\
037\_scissors & 75.5 & 25.0 & 32.3 & 14.6  & 74.2 & 27.7 & \textbf{97.8} & \textbf{95.5} &\textbf{97.4}	& \textbf{94.7} & 9.5 & 5.8 & 75.5 & 0.0 & 92.6 & 84.7 \\
040\_large\_marker &81.8 & 38.9 & 20.7 & 8.4 &  97.4 & 74.2 & \textbf{98.6} & \textbf{96.5} & \textbf{92.7} &	90.4& 9.1 & 8.0 & 79.6 & 39.3 & \textbf{96.5}& \textbf{91.0}\\
051\_large\_clamp & 83.0 & 34.4 & 24.1 & 11.2 & 82.7 & 34.7 & \textbf{96.9} & \textbf{92.7} & 87.4 & 68.9 & 22.4 & 8.2 &  \textbf{100.0} &  \textbf{100.0} & 92.9 & 84.2\\
052\_extra\_large\_clamp &  72.9 & 24.1 & 15.0 & 1.8 & 65.7 & 10.1 & \textbf{97.6} & \textbf{94.1} & \textbf{90.5} & 43.7 & 16.9 & 8.1 & 82.6 & 0.0 & 89.5 &  \textbf{65.8}\\
061\_foam\_brick &  79.2 & 35.5 & 59.4 & 31.4 & 95.7 & 45.8 & \textbf{98.1} & \textbf{93.4} & \textbf{98.7}	& 90.9 & 11.3 & 9.1 & 95.2 & 43.5 & 97.6 & \textbf{95.9}\\
\midrule
mean & 71.0 & 24.3 & 52.5 & 26.2 & 88.4 & 42.1 & \textbf{97.4} & \textbf{91.5} & 90.4 &76.1& 13.3 & 7.4 & 86.0 & 25.1 & \textbf{93.7} & \textbf{84.4}\\
         \bottomrule
    \end{tabular}
    \label{tab:ycbv_data_full}
    \vspace{0.2cm}
\end{table*}

\subsection{Full Tracking Results on YCB-Video Sequences}
We present the object tracking results on the full YCB-Video Sequences \cite{xiang2017posecnn} , using the first frame as the reference, in Table \ref{tab:ycbv_tracking_full}. We compare our approach with other CAD model-based novel object pose tracking methods, including \cite{wuthrich2013probabilistic}, RGF \cite{issac2016depth}, ICG \cite{stoiber2022iterative}, and FoundationPose \cite{wen2024foundationpose}. Our method achieves the best performance among one-view-based tracking methods and performs comparably to CAD model-based approaches.

\begin{table*}[]
    \centering
            \footnotesize
        \setlength{\tabcolsep}{2mm}
            \caption{Performance on pose tracking task. We compared with CAD model based tracking methods on YCB-V full video sequences. For our method, we still only give the first frame as a reference, and we keep the reference during tracking.}
    % \vspace{-0.3cm}
    \begin{tabular}{c|c c|c c|c c|c c||c c| c c }
        \toprule
        \textbf{Method}   & \multicolumn{2}{c|}{\textbf{Wuthrich}\cite{wuthrich2013probabilistic}} & \multicolumn{2}{c|}{\textbf{RGF}\cite{issac2016depth}} & \multicolumn{2}{c|}{\textbf{ICG}\cite{stoiber2022iterative}} & \multicolumn{2}{c|}{\textbf{FoundationPose}\cite{wen2024foundationpose}} & \multicolumn{2}{c||}{\textbf{FoundationPose}\cite{wen2024foundationpose}} & \multicolumn{2}{c}{\textbf{One2Any(Ours)}}\\

        Method & \multicolumn{2}{c|}{CAD} & \multicolumn{2}{c|}{CAD}  & \multicolumn{2}{c|}{CAD} & \multicolumn{2}{c||}{16 frames-CAD} & \multicolumn{2}{c|}{$1^{st}$ frame-CAD} & \multicolumn{2}{c}{$1^{st}$ frame} \\
                \midrule
        % Model-based &  \multicolumn{2}{c|}{ \checkmark} & \multicolumn{2}{c|}{ \xmark} & \multicolumn{2}{c|}{ \checkmark} & \multicolumn{2}{c|}{ \xmark} & \multicolumn{2}{c|}{ \xmark} & \multicolumn{2}{c}{ \xmark}\\
        metrics & ADD & ADD-S & ADD & ADD-S & ADD & ADD-S & ADD & ADD-S & ADD & ADD-S &   ADD & ADD-S\\
     \midrule
002\_master\_chef\_can & 55.6 & 90.7 & 46.2 & 90.2 & 66.4 & 89.7  & \textbf{91.2} & \textbf{96.9} & 38.1 &	83.3	& \textbf{83.8} & \textbf{94.8} \\
        003\_cracker\_box & 96.4 & 97.2 & 57.0 & 72.3 & 82.4 & 92.1  & \textbf{96.2} & \textbf{97.5}  & 78.3	& \textbf{94.0}& \textbf{83.0}	& 91.3 \\
        004\_sugar\_box & 97.1 & 97.9 & 50.4 & 72.7 & \textbf{96.1} & \textbf{98.4}  & 94.5 & 97.4 & 40.0	& 78.7 & \textbf{88.7} & \textbf{95.3} \\
        005\_tomato\_soup\_can & 64.7 & 89.5 & 72.4 & 91.6 & 73.2 & 97.3 & \textbf{94.3} & \textbf{97.9} & 14.0	& 49.3&  \textbf{87.1} 	&  \textbf{95.5} \\
        006\_mustard\_bottle   & 97.1 & 98.0 & 87.7 & 98.2 & 96.2 & 98.4 & \textbf{97.3} & \textbf{98.5} & 24.8	& 58.8	 & \textbf{87.7} &  \textbf{93.8}\\
        007\_tuna\_fish\_can  & 69.1 & 93.3 & 28.7 & 52.9 & 73.2 & 95.8  & \textbf{84.0} & \textbf{97.8} & 75.3	&\textbf{ 97.4}	& \textbf{89.5} & 95.9 \\
        008\_pudding\_box & 96.8 & 97.9 & 12.7 & 18.0 & 73.8 & 88.9  & \textbf{96.9} & \textbf{98.5} &\textbf{ 96.9}	&\textbf{98.3} & 93.5	& 96.3\\
        009\_gelatin\_box  & 97.5 & 98.4 & 49.1 & 70.7 & 97.2 & \textbf{98.8} & \textbf{97.6} & 98.5 & \textbf{97.2}	&\textbf{98.6} &  96.1	&97.7 \\
        010\_potted\_meat\_can  & 83.7 & 86.7 & 44.1 & 45.6 & 93.3 & 97.3 & \textbf{94.8} & \textbf{97.5} & 5.5	&52.6 & \textbf{65.9}	&\textbf{84.0}\\
        011\_banana  & 86.3 & 96.1 & 93.3 & 97.7 & \textbf{95.6} & \textbf{98.4} & \textbf{95.6} & 98.1 &64.7&	84.7 & \textbf{ 83.6}	&\textbf{95.1}  \\
        019\_pitcher\_base  & 97.3 & 97.7 & 97.9 & 98.2 & \textbf{97.0} & \textbf{98.8}  & 96.8 & 98.0 & \textbf{94.6}	&\textbf{96.4}	&  87.0 &93.4 \\
        021\_bleach\_cleanser  & 95.2 & 97.2 & 95.9 & 97.3 & 92.6 & \textbf{97.5} & \textbf{94.7} & \textbf{97.5} & 16.6 &	58.6& \textbf{ 84.8} &	\textbf{93.2} \\
        024\_bowl  & 30.4 & 97.2 & 24.2 & 82.4 & 74.4 & \textbf{98.4} & \textbf{90.5} &95.3 & 12.4&	40.2 & \textbf{71.8} &\textbf{91.8}\\
        025\_mug & 83.2 & 93.3 & 60.0 & 71.2 & \textbf{95.6} & \textbf{98.5} &91.5 & 96.1&54.4&	91.3	 & \textbf{83.3} &\textbf{95.5}\\
        035\_power\_drill & 97.1 & 97.8 & 97.9 & 98.3  & 96.7 & 98.5&\textbf{ 96.3} & \textbf{97.9} &50.4	&69.2 & \textbf{85.5} 	&\textbf{92.8} \\
        036\_wood\_block & 95.5 & 96.9 & 45.7 & 62.5 & \textbf{93.5} & \textbf{97.2} & 92.9& 97.0&  \textbf{88.4}	& \textbf{95.9}	& 85.5 &92.8\\
        037\_scissors & 4.2 & 16.2 & 20.9 & 38.6 & 93.5 & 97.3 & \textbf{95.5} & \textbf{97.8} & \textbf{96.0}	&\textbf{97.9} & 81.0	&91.7 \\
        040\_large\_marker & 35.6 & 53.0 & 12.2 & 18.9 & 88.5 & 97.8 & \textbf{96.6} & \textbf{98.6} & 74.0	&90.3 &\textbf{90.3}	&\textbf{96.2}  \\
        051\_large\_clamp  & 61.2 & 72.3 & 62.8 & 80.1 &91.8 &\textbf{96.9} & \textbf{92.5}& 96.7&60.1&	81.0 & \textbf{84.5} & \textbf{93.2} \\
        052\_extra\_large\_clamp  & 93.7& 96.6 & 67.5 & 69.7 & 85.9 & 94.3& \textbf{93.4} & \textbf{97.3}& 44.4	&85.1 & \textbf{71.1}	&\textbf{91.0} \\
        061\_foam\_brick  & 96.8 & 98.1 & 70.0& 86.5 & 96.2 & \textbf{98.5}  & \textbf{96.8} & 98.3 &  89.8&	\textbf{98.2}&	 \textbf{96.1} & 97.7 \\
        \midrule
        mean  & 78.0 & 90.2 & 59.2 & 74.3 & 86.4 & 96.5 & \textbf{93.7} & \textbf{97.5} & 57.9	&80.9	& \textbf{84.8} & \textbf{93.8} \\
        \bottomrule
    \end{tabular}
    \label{tab:ycbv_tracking_full}
    \vspace{0.2cm}
\end{table*}

% \noindent{}\textbf{Pose tracking results on Real275 test set. } We further test the pose tracking performance on Real275 \cite{wang2019normalized}. Results are presented in Table \ref{tab:pose_tracking_nocs}. We compare with Oryon \cite{corsetti2024open} and FoundationPose \cite{wen2024foundationpose} given always the first frame of the test set. Furthermore, we measure the average precision of predicted poses that are with $5\degree5cm, 10\degree5cm$ threshold. Note that, this is a quite strict metrics to measure the pose estimation performance, and we roughly call the poses within the threshold as the 'correct' poses. We tested all 18 objects that belong to 6 categories in Table \ref{tab:pose_tracking_nocs}. We observe that for some objects, FoundationPose failed to estimate the 'correct' poses in bowl, camera, laptop and mugs.

\subsection{Robustness Analysis on the Selection of Reference Images}
To further demonstrate the robustness of One2Any on the selection of different reference images, we additionally measure the standard deviation of the method when dealing with different reference images. We conducted experiments following Oryon~\cite{corsetti2024open}, evaluating 2000 randomly selected reference-query image pairs from the Real275~\cite{wang2019normalized} and Toyota-Light~\cite{hodan2018bop} datasets respectively. These datasets contain various combinations of the same objects
with different reference-query pairs. As shown in Table 1 (main paper), our method significantly outperforms existing approaches when handling different reference images. To further analyze robustness, we computed the standard deviation (std) for each object and averaged
them (see in Table~\ref{tab:different_ref_images}). Our method achieves a lower std, demonstrating its robustness to variations in reference images. 
\begin{table}[]
    \centering
        \footnotesize
        \setlength{\tabcolsep}{3mm}
    \captionof{table}{Robustness Analysis. We measure the standard deviation (std) of AR score and ADD-AUC metrics.}
                % \vspace{-0.3cm}
\begin{tabular}{l | c c | c c}
    \toprule
       \multirow{2}{*}{Methods} & \multicolumn{2}{c|}{Real275~\cite{wang2019normalized}} & \multicolumn{2}{c}{Toyota-Light~\cite{hodan2018bop}} \\
         & AR & ADD-AUC & AR & ADD-AUC\\
         \midrule
        % Oryon mean & 46.5 & 34.9 & 34.1 &22.9\\
        Oryon~\cite{corsetti2024open} std & 25.7 & 46.9  & 25.6 & 42.3\\
        \midrule
        % One2Any mean& 54.9 & 41.0 & 42.0 & 34.6 \\
        One2Any std & \textbf{15.6} & \textbf{27.2}  & \textbf{22.5} & \textbf{30.5} \\
        \bottomrule
    \end{tabular}
    \label{tab:different_ref_images}
\end{table}

\subsection{Performance on Occluded Scenes} 
For scenes with occlusions—whether in the reference image or the test image—our method demonstrates strong robustness in handling occluded scenarios, where other methods often fail. Detailed results are presented in Figure \ref{fig:occlusion}.

We observe that occlusions lead to incorrect correspondences in Oryon \cite{corsetti2024open}, causing significant translation errors. This results in a projected pose that is far from the ground truth, as illustrated in row 1, where the predicted pose is projected entirely out of the image. Similarly, NOPE \cite{nguyen2024nope} struggles with occlusions in the reference image. In such cases, suboptimal feature extraction leads to incorrect relative pose predictions in the latent space, as seen in rows 1–3. However, when the reference image provides clear, representative texture input (row 4), NOPE can handle pose estimation effectively, even if the test image is occluded.  FoundationPose \cite{wen2024foundationpose}, on the other hand, heavily depends on the quality of its generated model. Figure \ref{fig:occlusion} shows two views of the generated model: the upper view resembles the reference image, while the lower view corresponds to the test image. When the test view aligns well with the generated CAD model, FoundationPose performs reliably. However, when the test view deviates significantly from the generated model, as seen in rows 2 and 4, it fails to predict the correct pose.

In contrast, our method is highly robust to occlusions in both the reference and test images, consistently achieving accurate pose estimation even under challenging conditions.

\begin{figure}
    \centering
    \includegraphics[width=1.0\linewidth]{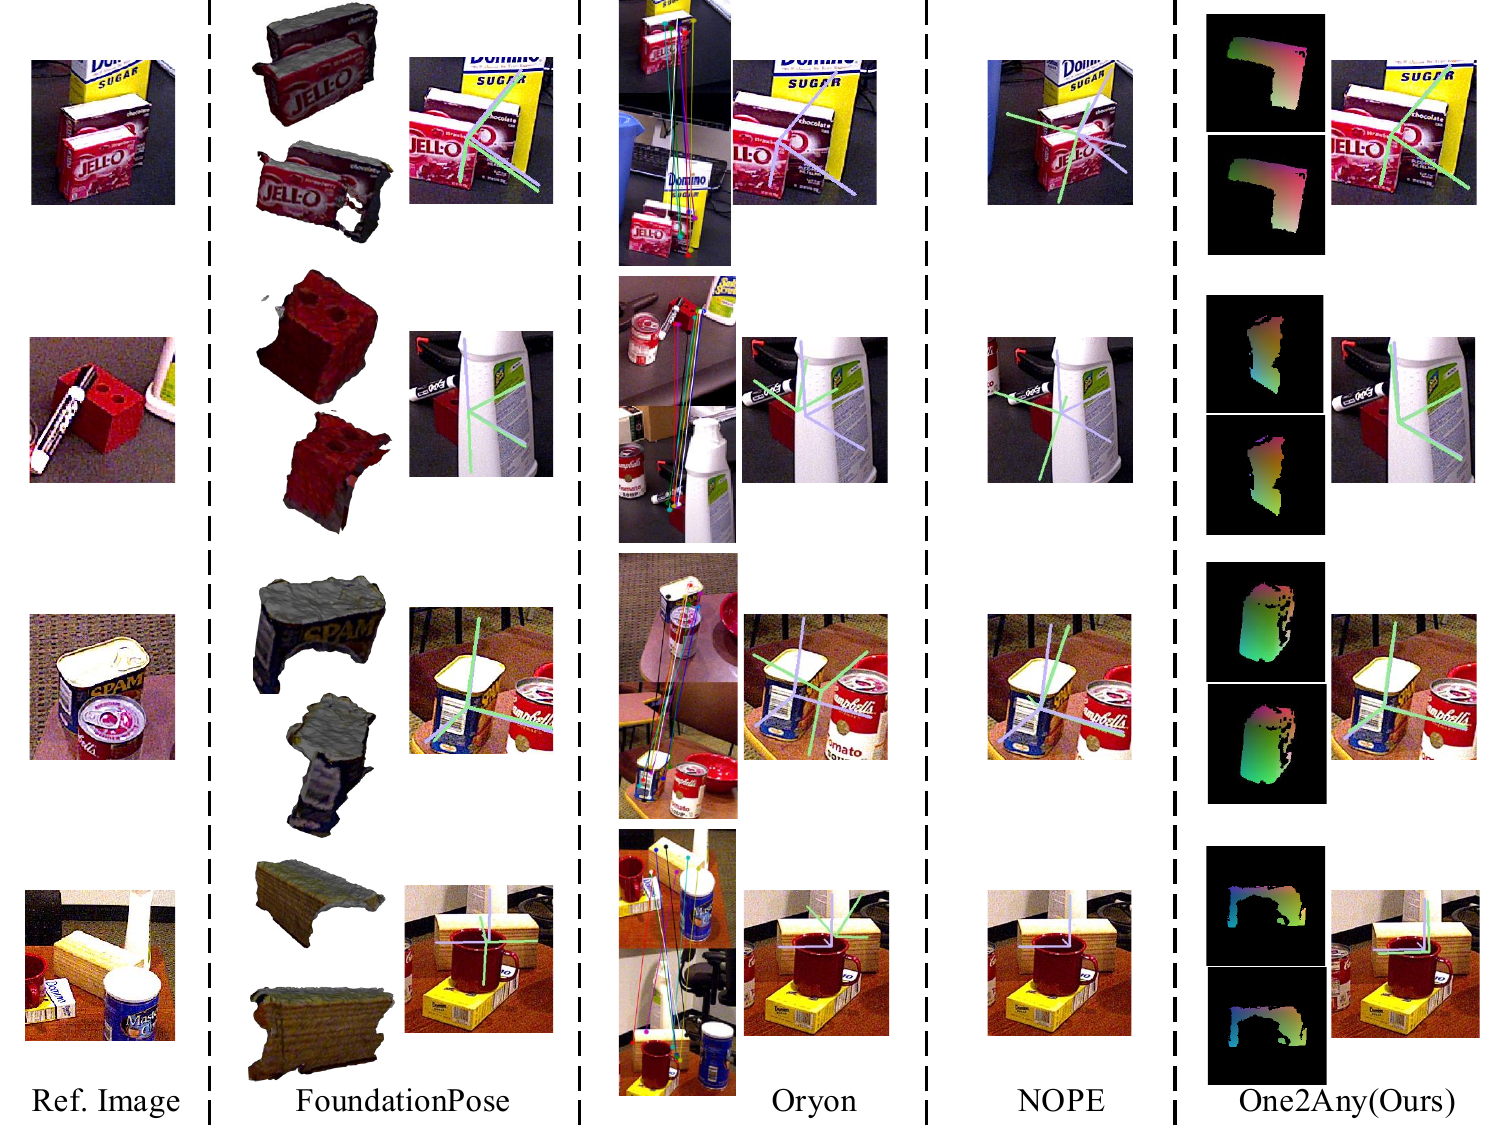}
    \caption{Qualitative results on occluded scenes. We present results for scenarios where occlusion occurs in the reference image and the test image, respectively. The test image displays projected poses with axes, where the green color represents the predicted pose, and the pink color indicates the ground-truth pose. For FoundationPose \cite{wen2024foundationpose}, we also include the generated model derived from the reference image. The upper model view corresponds to the reference image, while the lower model view aligns with the test image. For Oryon \cite{corsetti2024open}, we visualize its predicted correspondences. For One2Any (Ours), we additionally compare the generated ROC map (below) with the ground-truth ROC map (above). }
    \label{fig:occlusion}
\end{figure}

\subsection{Performance on Large View Variations} 
We show qualitative results for scenes with significant view variations in Figure \ref{fig:view_variation}. These scenarios involve objects with markedly different perspectives in the reference and test images. Even in the absence of occlusion, low overlap between the object views presents a significant challenge for pose estimation when only a single reference view is provided.

Methods based on correspondences often fail in such cases due to the difficulty of establishing accurate matches. Similarly, the latent space searching approach used by NOPE \cite{nguyen2024nope} performs poorly when it is unable to conduct a comprehensive search in the latent space. For model-based methods, the effectiveness of the generated model can degrade under such conditions. As shown in the last two rows, only partial regions of the object are generated from the reference image, resulting in poor supervision for pose estimation when the test view has minimal overlap with the reference.

In contrast, One2Any performs robustly even with large view variations. This stability is attributed to the model’s ability to predict ROC maps, effectively inferring missing parts of the object given the Reference Object Embedding (ROPE) and ensuring accurate pose predictions.

\begin{figure}
    \centering
    \includegraphics[width=1.0\linewidth]{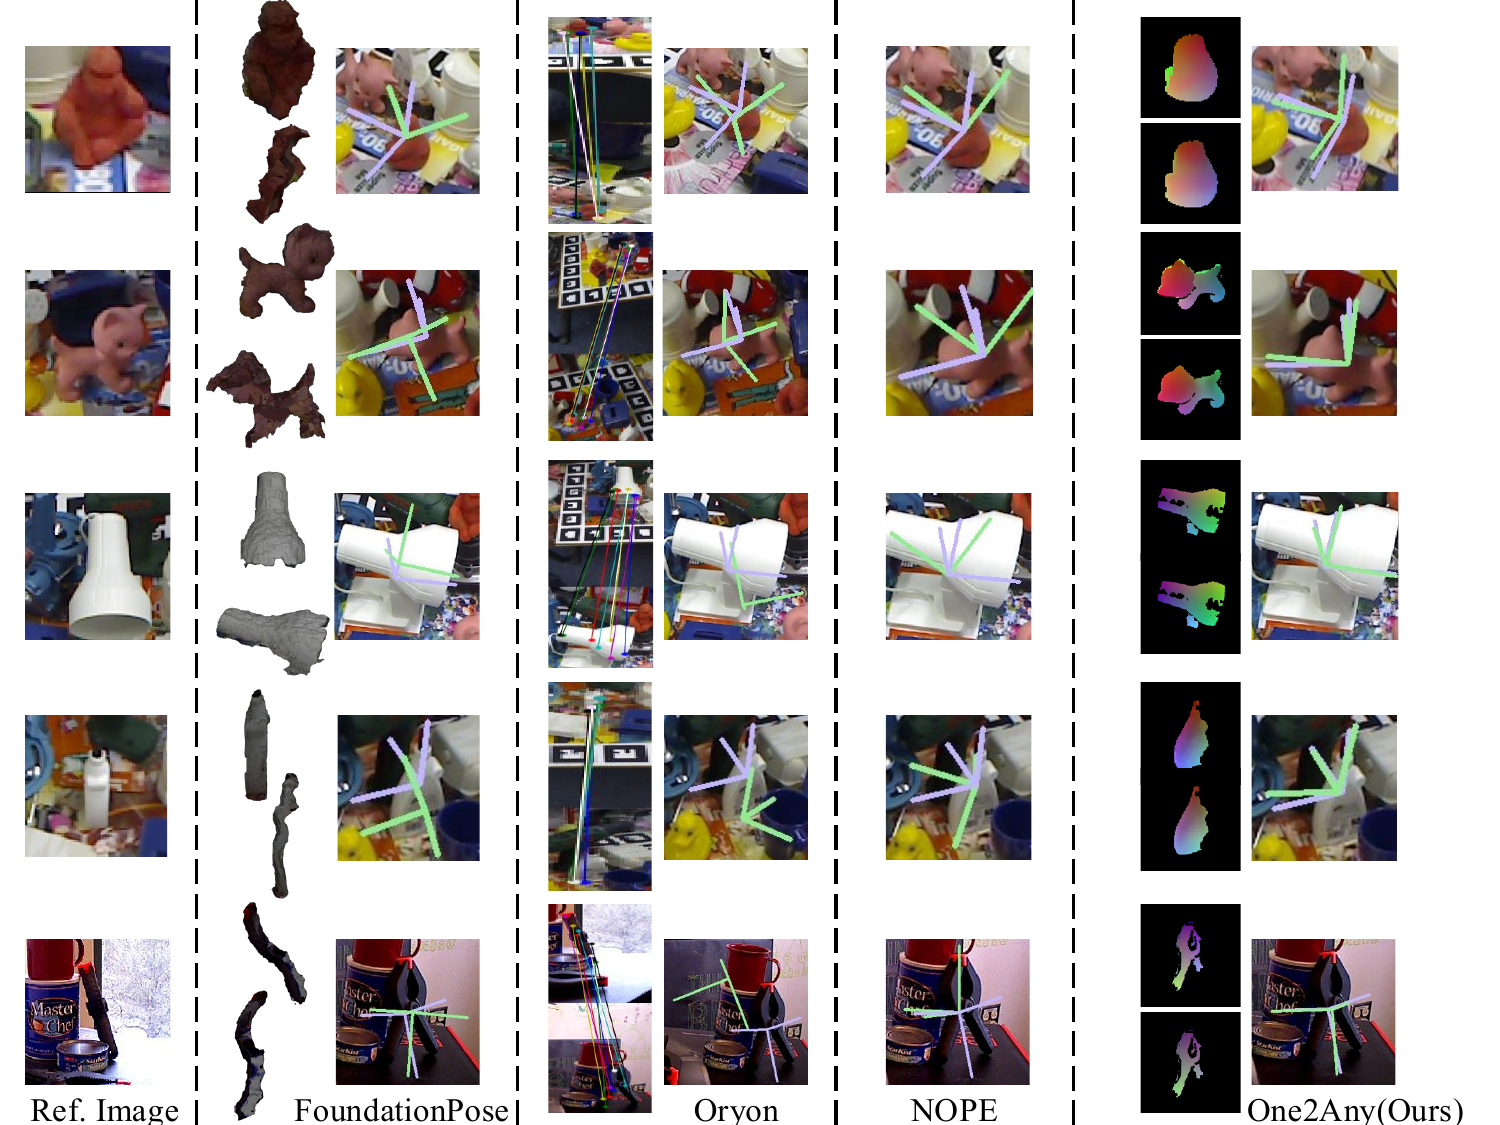}
    \caption{Qualitative results on large view variations. We present results for scenarios with significant view variations, including cases with low or almost no overlap between the reference and test images. In the test images, we display the projected poses with axes, where the green color represents the predicted pose and the pink color indicates the ground-truth pose. For FoundationPose \cite{wen2024foundationpose}, we also include the generated model derived from the reference image. The upper view corresponds to the reference image, while the lower view aligns with the test image. For Oryon \cite{corsetti2024open}, we visualize its predicted correspondences. For One2Any (Ours), we additionally show the generated ROC map (below) alongside the ground-truth ROC map (above).}
    \label{fig:view_variation}
\end{figure}

\subsection{Performance on Textureless Objects} 
We further present additional results for textureless objects in Figure \ref{fig:textureless}. Textureless objects are known to introduce significant challenges for correspondence matching and template matching methods. As a result, these approaches often fail to predict accurate poses for textureless objects. For example, Oryon \cite{corsetti2024open} struggles with large translation errors, leading to projections that fall outside the image frame.

In contrast, our method, which predicts poses through ROC map generation, demonstrates stability and robustness in handling textureless objects, maintaining accurate pose predictions even under these challenging conditions.

\begin{figure}
    \centering
    \includegraphics[width=1.0\linewidth]{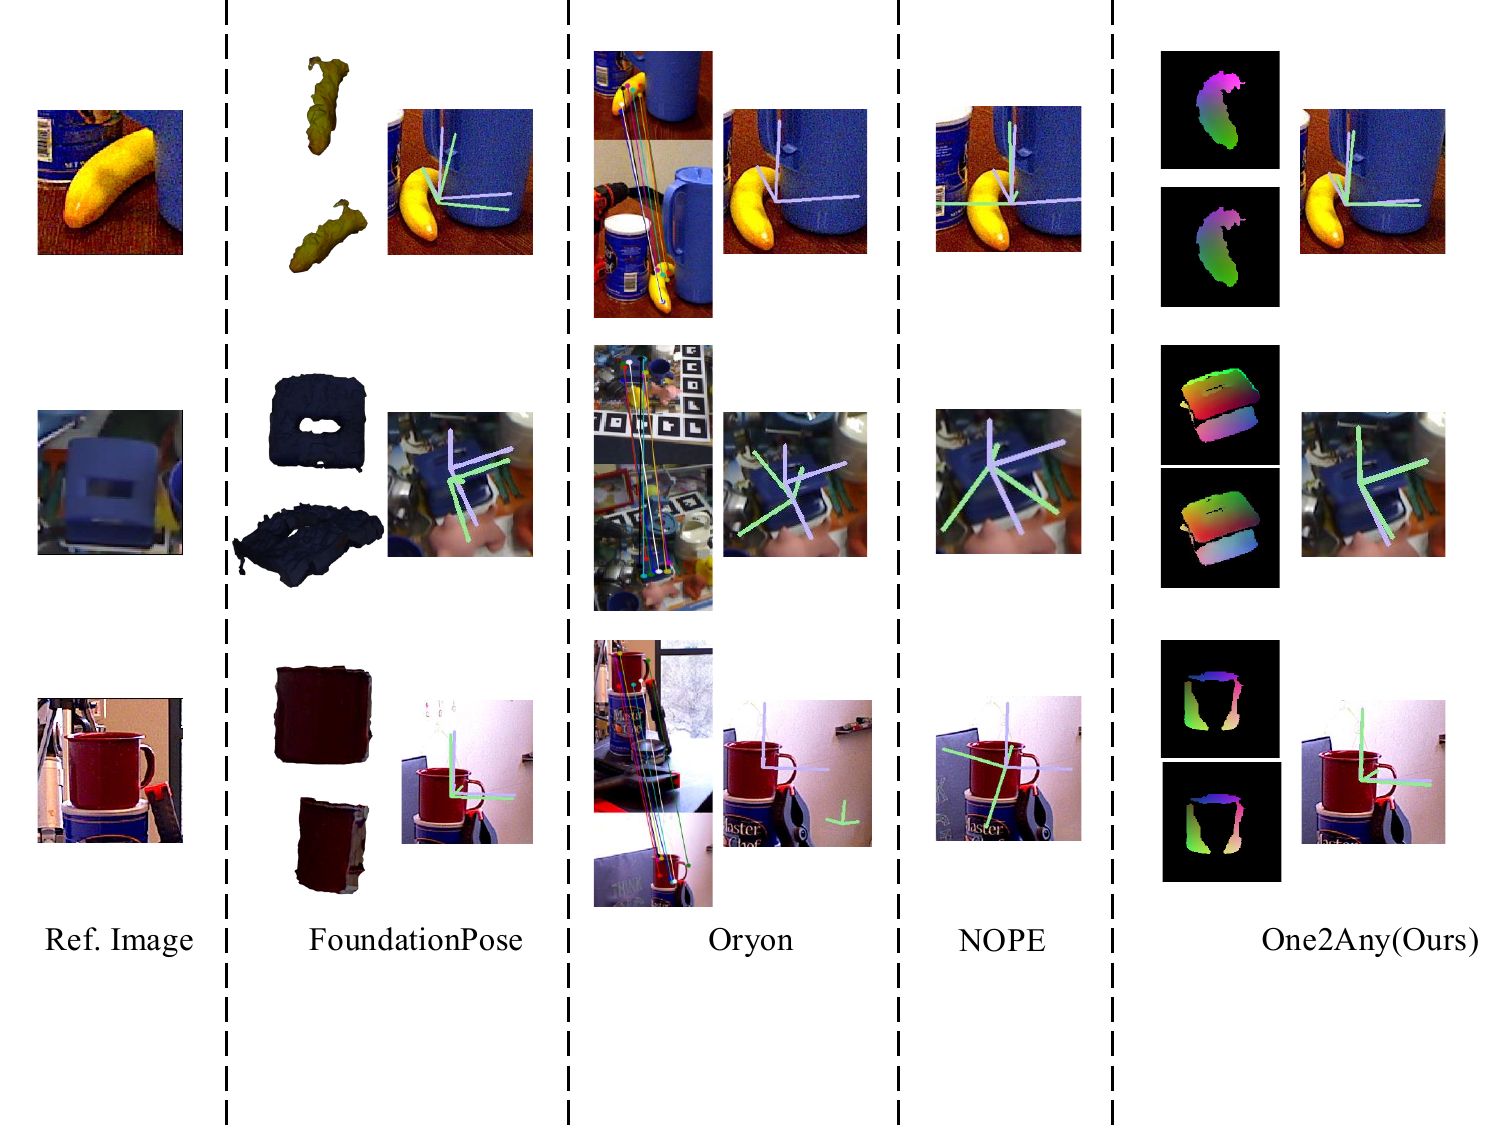}
    \caption{Qualitative results on textureless objects. We evaluate the pose estimation performance for textureless objects, which is presented in Figure \ref{fig:textureless}. The test images display projected poses with axes, where the green color represents the predicted pose and the pink color indicates the ground-truth pose. For FoundationPose \cite{wen2024foundationpose}, we include the generated model derived from the reference image. The upper view corresponds to the reference image, while the lower view aligns with the test image. For Oryon \cite{corsetti2024open}, we visualize its predicted correspondences. For One2Any (Ours), we additionally compare the generated ROC map (below) with the ground-truth ROC map (above).}
    \label{fig:textureless}
\end{figure}

\subsection{More Qualitative Results on Novel Objects}
We present additional qualitative results of our method across various test datasets, including YCB-Video \cite{xiang2017posecnn}, Toyota-Light \cite{hodan2018bop}, T-LESS \cite{hodan2017t}, IC-BIN \cite{doumanoglou2016recovering}, and TUD-L \cite{hodan2018bop}. These datasets are popular in the BOP benchmark. The results are illustrated in Figure \ref{fig:more_visualization}, where we also display the predicted ROC map alongside the reference ROC map.

Our method demonstrates the ability to predict poses for a diverse range of unseen objects across different datasets, such as an unusual toy dinosaur and a charger. Additionally, our method is robust to challenging conditions like significant lighting changes. For instances with large view variations and minimal overlap, such as the cup example, our method accurately estimates the pose.

We also showcase pose tracking performance with the driller object, where our method successfully follows the object’s motion and achieves accurate pose tracking using only the first view as a reference. The processing time is approximately 0.09 seconds per frame with a single Nvidia RTX 4090 GPU.
\begin{figure}
    \centering
    \includegraphics[width=1.0\linewidth]{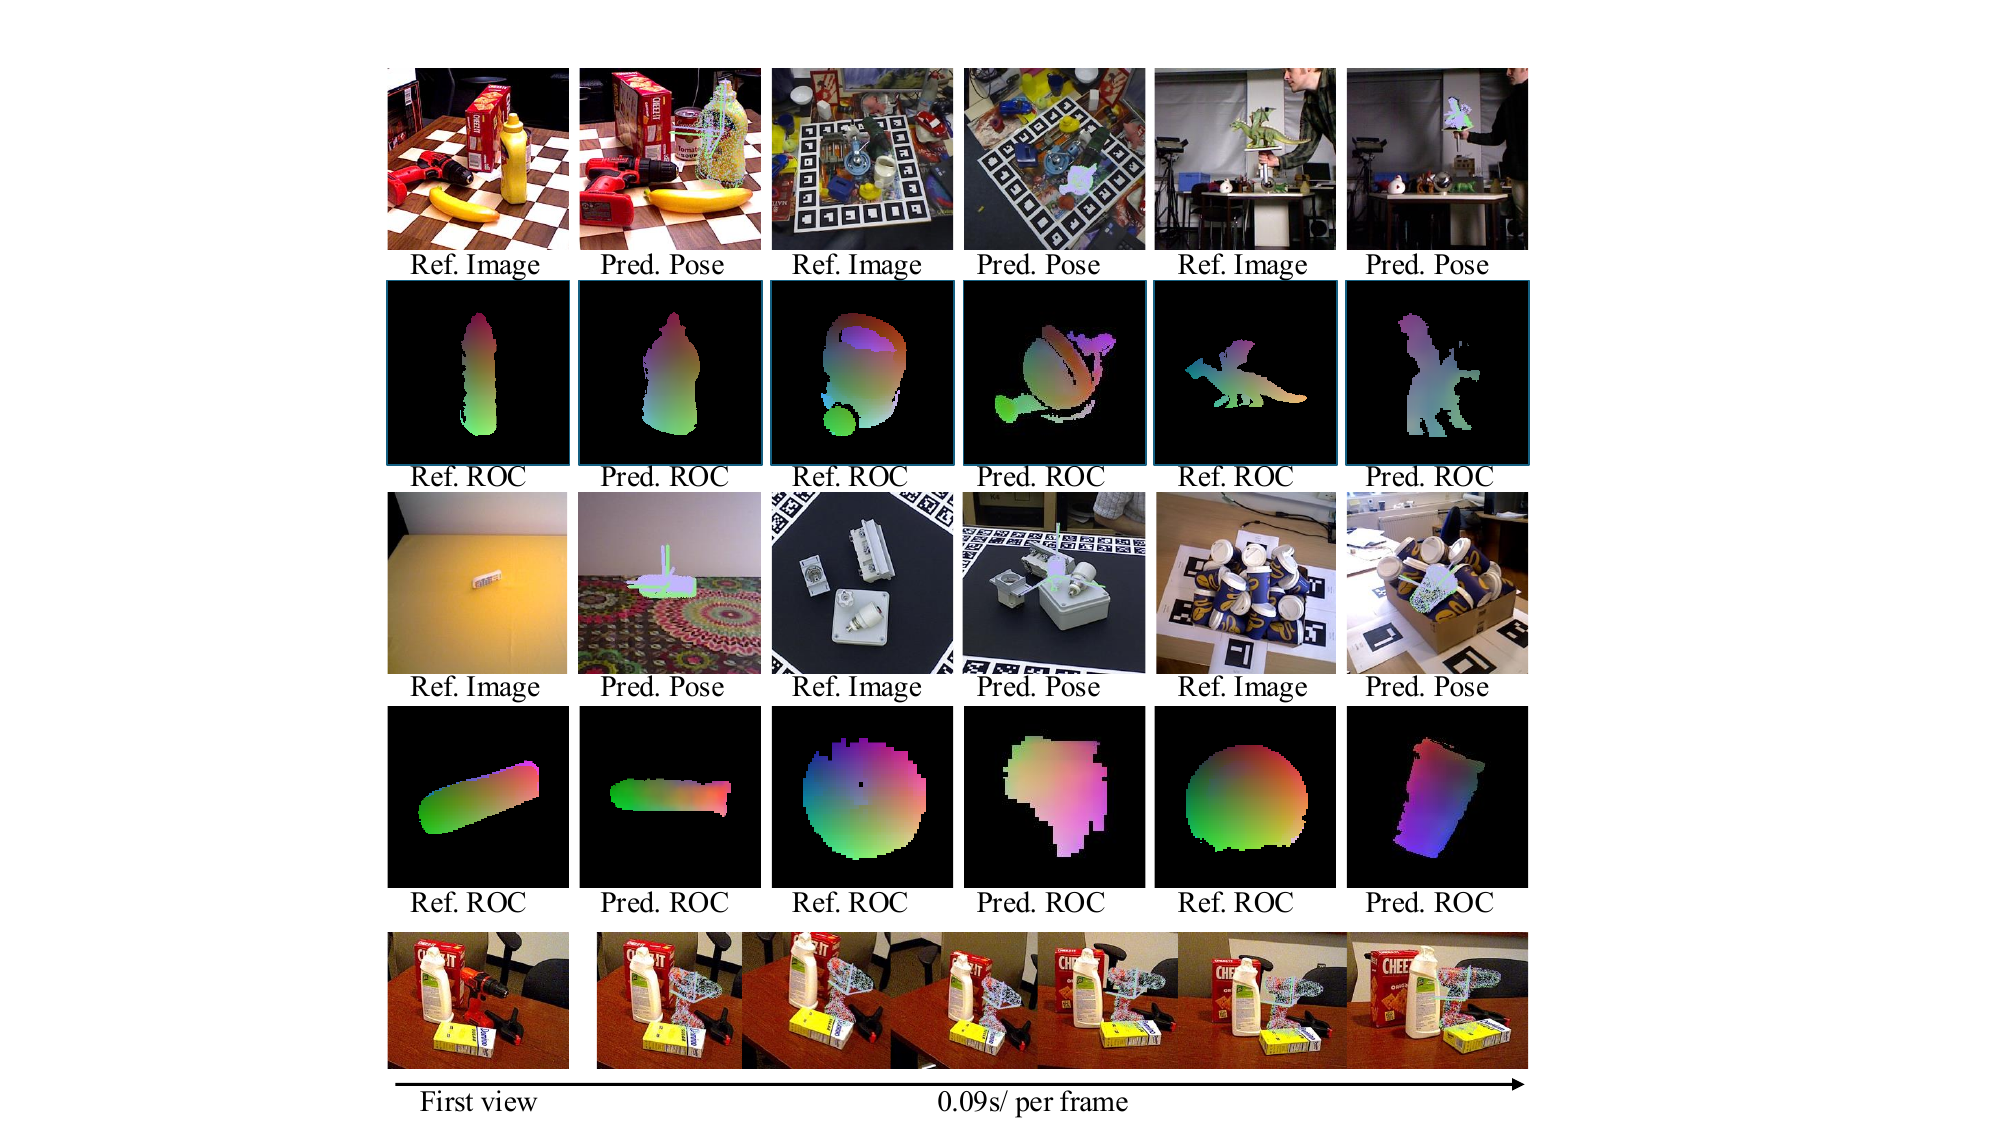}
    \caption{More qualitative results. We present pose estimation results across additional test datasets, including YCB-Video \cite{xiang2017posecnn}, Toyota-Light \cite{hodan2018bop}, T-LESS \cite{hodan2017t}, IC-BIN \cite{doumanoglou2016recovering}, and TUD-L \cite{hodan2018bop}. For each dataset, we display the ROC maps for the reference images and the predicted ROC maps for the test images. Furthermore, we demonstrate the tracking performance on the YCB-Video dataset. The predicted pose is shown in green, while the ground-truth pose is shown in pink. Additionally, we present the projections of the object point cloud on the image, corresponding to both the ground-truth pose and the predicted pose. }
    \label{fig:more_visualization}
\end{figure}

\subsection{Experiments with RGB-only Inputs} To further explore the ability of One2Any when dealing with RGB query images only (without depth inputs), we use RANSAC+PnP~\cite{fischler1981random}
for pose estimation and tested on YCB-Video~\cite{xiang2017posecnn}. Results are shown in Table~\ref{tab:pose_compute}, we measure the average rotation error and translation error for detailed comparison. RGB-only input achieves competitive rotation estimation, even outperforming Umeyama~\cite{umeyama1991least}. However, estimating translation from a single view without depth is inherently challenging, as depth provides critical scale information. For instance, NOPE~\cite{nguyen2024nope}, a single view method which uses RGB-only input, does not estimate translation at all.

\begin{table}[]
       \centering
    \footnotesize
       \setlength{\tabcolsep}{1.5mm}
      \captionof{table}{Performance of PnP method~\cite{fischler1981random} (without depth input) compared with Umeyama algorithm ~\cite{umeyama1991least} (with depth input). We test on YCB-V test set and measure the rotation error and translation error in detail.}
                       % \vspace{-0.3cm}
    \begin{tabular}{c|c c} % c c}
    \toprule
        Method & rotation err (°) & translation err (m)\\ % & ADD-S & ADD  \\
        \midrule
       Umeyama~\cite{umeyama1991least}  &  22.2 & \textbf{0.02} \\ %& \textbf{93.7} & \textbf{84.4}\\
       RANSAC+PnP~\cite{fischler1981random} &  \textbf{21.0} & 0.04 \\%& 76.4 & 51.6 \\
       \bottomrule
    \end{tabular}
        \label{tab:pose_compute}
\end{table}

\subsection{Training Data Scalability}
\label{sec:training_scale}
We evaluate the impact of training data size on our method. Due to the simplicity of our data collection process—requiring only image pairs of the same object—we can generate an unlimited amount of synthetic data for training. To analyze the effect of training data scale, we gradually increase the size of the training dataset and evaluate performance on the  consistently used test set YCB-Video \cite{xiang2017posecnn}  test set as the evaluation benchmark. The metrics used are ADD-AUC and ADD-S AUC, with results presented in Figure \ref{fig:training_data}.

For comparison, we include performance from FoundationPose \cite{wen2024foundationpose}. Our observations show that the performance of our method improves steadily with an increasing amount of training data. Notably, when the training data size increases to 1M, FoundationPose shows little to no improvement, whereas our method continues to demonstrate significant gains. This indicates that the performance of our approach can be further enhanced with even larger datasets. Due to computational resource limitations, we capped the training data size at approximately 2M samples.

\begin{figure}
    \centering
    \includegraphics[width=0.8\linewidth]{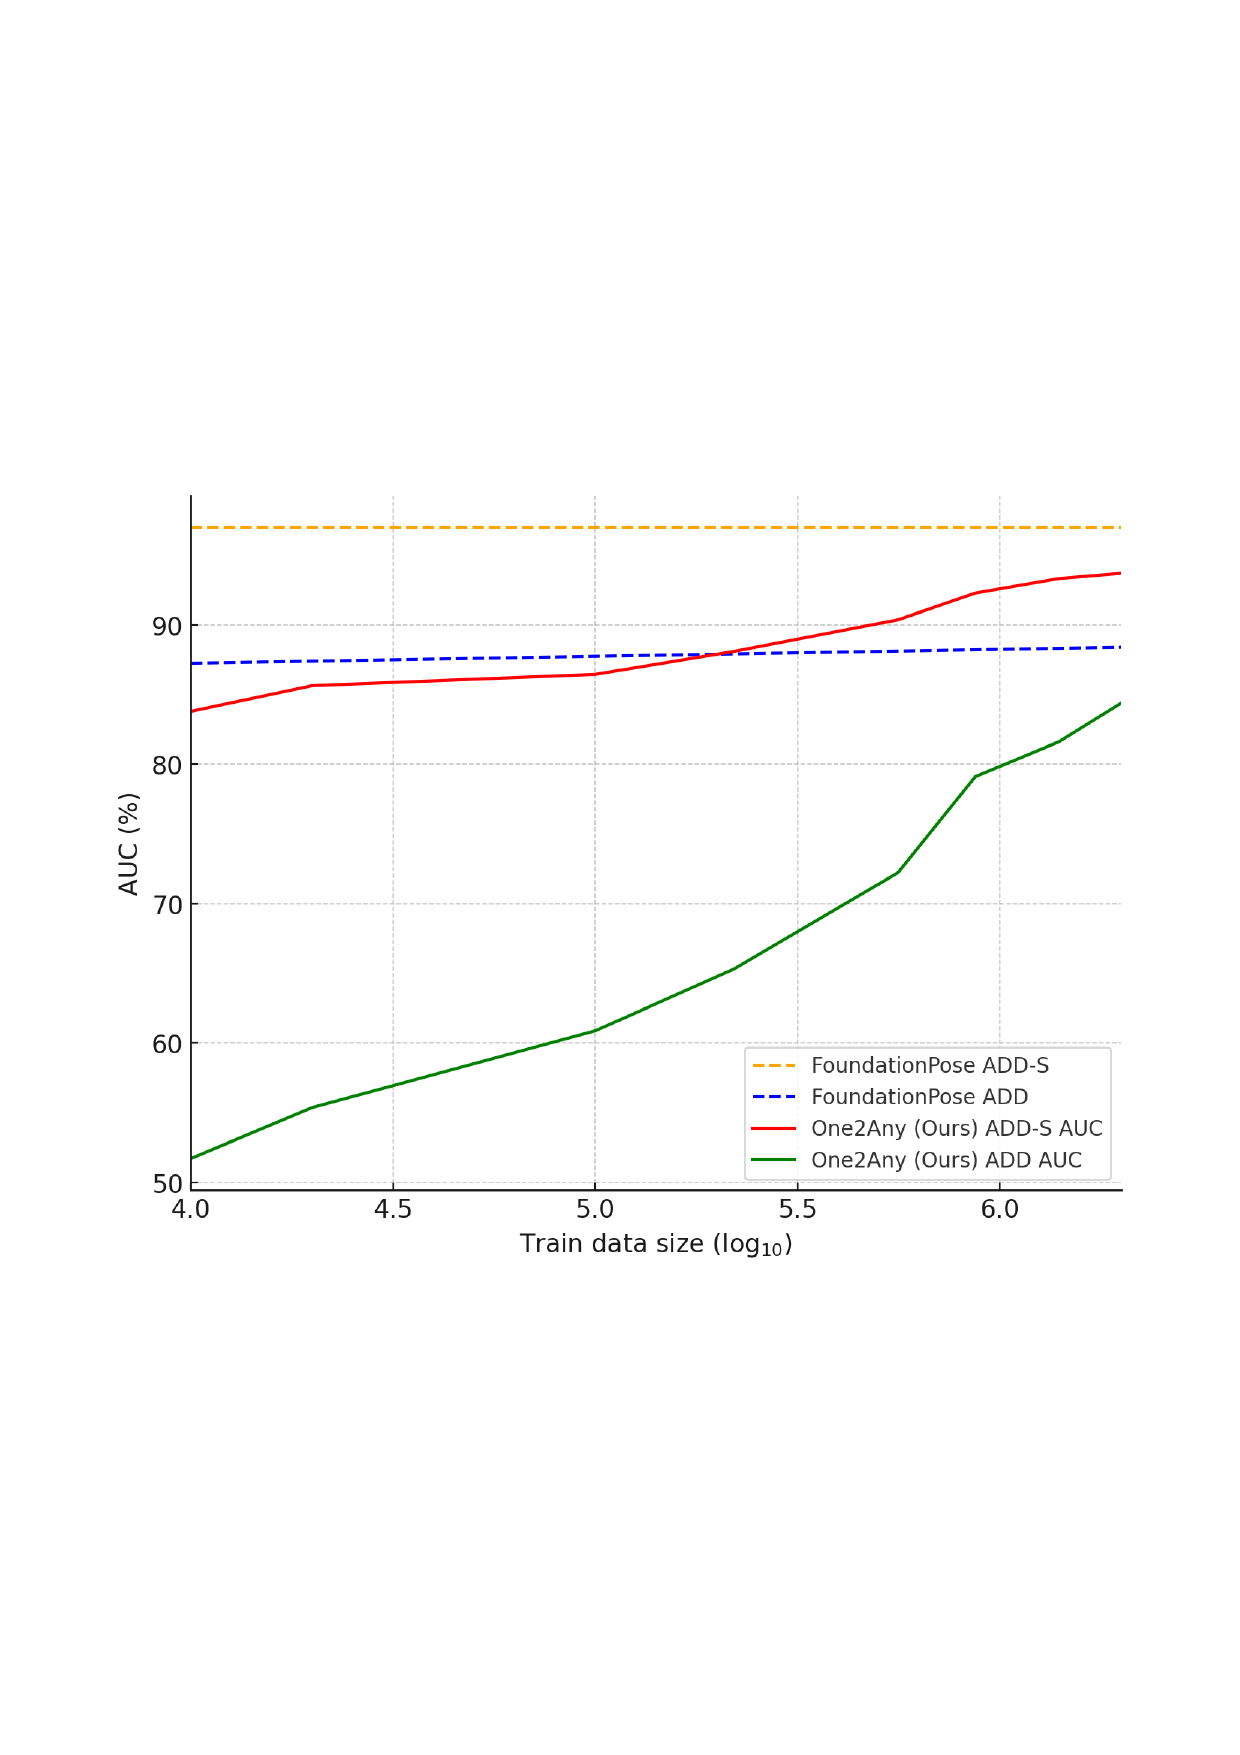}
    \caption{Training data scalability. We analyze the effect of training data size on our method’s performance and compare it with FoundationPose \cite{wen2024foundationpose}.}
    \label{fig:training_data}
\end{figure}
