# Supplementary material for: One2Any: One-Reference 6D Pose Estimation for Any Object
Source: arXiv:2505.04109 source file (2025-05-07)
Supplement: Supplementary file 3 [file 3_extension_to_multiview_setups.tex]

\section{Extension to Multi-view Setups}
\label{sec:multiview_setups}

We further extend our method to multi-view setups. Owing to its time efficiency, our method can seamlessly handle multi-view configurations by estimating the relative pose between the test image and each reference image in the multi-view set. The best prediction is then selected based on these estimations.

\subsection{Simple Voting Strategy for Pose Selection}
Assume we have  $N$  multi-view reference images, resulting in  $N$  predicted poses  $[\mathbf{R}|\mathbf{t}]_{i \in N}$. We employ a simple voting strategy to identify the optimal prediction among these poses.

When utilizing multi-view reference images, we assume low overlap between the images. Consequently, for each test image, there exists an optimal prediction corresponding to one of the reference views. The objective is to use a voting strategy based on reprojection error to identify this best match.

First, we filter out incorrect predictions using reprojection error. Given a predicted relative pose between the test image and reference image  $A_{I_i}$, we estimate the relative pose $[\hat{\mathbf{R}}|\hat{\mathbf{t}}]_{i2r}$, With the ground-truth pose of the reference view $[\mathbf{R}|\mathbf{t}]_{i}$. The predicted pose of the current test image is:
\begin{equation}
    [\hat{\mathbf{R}}|\hat{\mathbf{t}}]_i = [\hat{\mathbf{R}}|\hat{\mathbf{t}}]_{i2r} [\mathbf{R}|\mathbf{t}]_{i}
\end{equation}

Next, we compute the reprojection error from the test image to all reference images. Using the predicted pose, we obtain. We first get the point cloud $W_Q$ in the world coordinate with the predicted pose.
\begin{equation}
    W_Q = {[\hat{\mathbf{R}}|\hat{\mathbf{t}}]_i}^{-1}\mathbf{K}^{-1}Q_D[Q_M=1]
\end{equation}
$\mathbf{K} \in \mathbb{R}^{4\times4}$ is the camera intrinsic matrix, $Q_D, Q_M$ are the depth image and the mask image respectively. Thus, for each reference image $A_j, j\in N$, we have 
\begin{equation}
   P_{A_j} = \mathbf{K}[\mathbf{R}|\mathbf{t}]_{j}W_Q
\end{equation}
Then we get the projected pixels in the image frame
\begin{equation}
        \begin{bmatrix} U \\ V\end{bmatrix}
 = \frac{P_{A_j}[:, :2]}{{P_{A_j}[:, 2]}} 
\end{equation}
And we get the projected mask as:
\begin{equation}
    \hat{A}_{M_j}[U \ V] = 1
\end{equation}
To evaluate the prediction, we compute the mIoU \cite{everingham2010pascal} between the predicted mask $ \hat{A}_{M_j}$ and the ground-truth mask  $A_{M_j}$. Typically, for each test image, there exists at least one reference image where the reprojection results in a high overlap with the ground-truth mask, yielding a high mIoU. However, for other reference images, the predicted mask may result in a lower IoU. Consequently, we select the predicted pose corresponding to the maximum IoU across all reference images as the final predicted pose.
% Thus, we set a threshold to 0.8 that if the IoU is over 0.8, we believe it's a reliable prediction on pose that it correctly project the seen part to one reference image.

% Furthermore, we notice there are some situations that the test image is not like any reference view, resulting its poor mIoU in all reference images. For this case, we simply use a cluster way to find the optimal pose. To be specific, we cluster the predicted poses and find the cluster that has the smallest difference inside, and choose the average pose over the cluster as our prediction.
\begin{table*}[]
\centering
    \footnotesize
    \setlength{\tabcolsep}{0.7mm}
    \caption{Performance on LINEMOD \cite{hinterstoisser2011multimodal} dataset with multi-view setups. We report the recall of ADD-0.1d metric. Results of multi-view methods are taken from FS6D~\cite{wen2024foundationpose}. The best performance among multi-view methods are highlighted in bold. One2Any(Ours) 8-view, 16-view methods are evaluated with a pose selection strategy, while 8-best view and 16-best view results are approached with the best prediction.}
    % \vspace{-0.2cm}
\begin{tabular}{l|c c| c c c c c c c c c c c c c|c}
\toprule
\textbf{Methods} & \textbf{Modality}  & \textbf{Ref. Images} & \textbf{ape} & \textbf{benchwise} & \textbf{cam} & \textbf{can} & \textbf{cat} &  \textbf{driller} & \textbf{duck} & \textbf{eggbox} & \textbf{glue} & \textbf{holepuncher} & \textbf{iron} & \textbf{lamp} & \textbf{phone} & \textbf{mean} \\
% \textbf{Method} & \textbf{ape}    & \textbf{cat} & \textbf{driller} & \textbf{duck} & \textbf{eggbox} & \textbf{glue}   & \textbf{iron} & \textbf{lamp} & \textbf{phone} & \textbf{Avg.} \\
\midrule
% Gen6D \cite{40} & RGB & \xmark & 200 & - & 77 & 66.1 & 62.8 & 60.7 & 67.4 & 40.5 & 95.7 & 87.2 & - & - & - & - & 63.6 \\
% Gen6D \cite{liu2022gen6d} & RGB & 200 & - & 62.1 & 45.6 & 64.7 & 40.9 & 48.8 & 16.2 & - & - & - & - & - & - & - \\
OnePose \cite{sun2022onepose} & RGB & 200 & 11.8 & 92.6 & 88.1 & 77.2 & 47.9 & 74.5 & 34.2 & 71.3 & 37.5 & 54.9 & 89.2 & 87.6 & 60.6 & 63.6 \\
OnePose++ \cite{he2022onepose++} & RGB  & 200 & 31.2 & 97.3 & 88.0 & 89.8 & 70.4 & 92.5 & 42.3 & 99.7 & 48.0 & 69.7 & \textbf{97.4} & \textbf{97.8} & 76.0 & 76.9 \\
LatentFusion \cite{park2020latentfusion} & RGBD & 16 &  \textbf{88.0} & 92.4 & 74.4 & 88.8 & 94.5 & 91.7 & 68.1 & 96.3 & 49.4 & 82.1 & 74.6 & 94.7 & 91.5 & 83.6 \\
% FS6D \cite{he2022fs6d} & RGBD & \xmark & 16 & 74.0 & 86.0 & 88.5 & 86.0 & 98.5 & 81.0 & 68.5 & 100.0 & 99.5 & 97.0 & 92.5 & 85.0 & 99.0 & 88.9 \\
FS6D \cite{he2022fs6d} + ICP & RGBD & 16 & 78.0 & 88.5 & 91.0 & 89.5 & \textbf{97.5} & 92.0 & 75.5 & 99.5 & 99.5 & \textbf{96.0} & 87.5 & 97.0 &\textbf{97.5} & 91.5\\
% FoundationPose \cite{wen2024foundationpose}& RGBD & 16-CAD & \textbf{99.9} & \textbf{100.0} & \textbf{100.0} & \textbf{100.0} &  \textbf{100.0} &\textbf{100.0}   & \textbf{99.4} & \textbf{100.0} & \textbf{100.0} & \textbf{99.9} & \textbf{100.0} & \textbf{100.0}& \textbf{100.0} & \textbf{99.9}\\
\midrule 
% % \midrule
% % FoundationPose & RGBD & \xmark & 16 & 99.0 & 100.0 & 100.0 & 100.0 & 100.0 & 100.0 & 99.4 & 100.0 & 100.0 & 99.9 & 100.0 & 100.0 & 100.0 & \textbf{99.9} \\
% % FoundationPose \cite{wen2024foundationpose}& RGBD & 1-CAD & \textbf{36.5} & \textbf{55.5} & \textbf{84.2} & \textbf{71.7} &  65.3 &16.3  & \textbf{49.8} & 42.6 & 64.8 & \textbf{52.7} & 20.7 & 15.8 & 51.7 & 48.3\\
% % NOPE \cite{nguyen2024nope} & RGB & 1 + GT trans & 2.0 & 4.5 &  2.5 & 2.2 & 0.7 & 4.7& 0.5 &  \textbf{100.0} & 79.4 & 2.9  & 4.5 & 4.2 & 3.9 &16.3\\
% % Oryon \cite{corsetti2024open} &  RGBD & 1 & 1.2 & 1.3 & 3.9 & 0.8 & 12.7  & 8.5 & 0.8 & 63.2 & 18.4 & 1.6 & 0.6 &2.9 & 11.7 & 9.8 \\
% \midrule
% % Ours & RGBD & \xmark & 1 & 43.4 & 59.3 & 59.7 & 59.3 & 54.4 & 65.7 & 35.8 & 100.0 & 99.9&  55.4 & 28.0 & 52.4 & 53.0 &  \\
% One2Any (Ours) & RGBD  & 1 & 33.1& 15.7 & 72.7 & 37.0 & \textbf{66.2}  & \textbf{68.2} & 35.8 & \textbf{100.0} & \textbf{99.9} &  42.0 & \textbf{28.2} & \textbf{31.9} & \textbf{53.2} & \textbf{52.6} \\
\midrule 
One2Any (Ours) & RGBD  & 8 & 79.9 & 75.1 & 88.5 & 60.6 & 90.1 & 70.5 & 45.8 & 100.0 & 99.9 & 84.4 & 60.7 & 84.0 & 89.9 & 79.2\\
One2Any (Ours) & RGBD  & 16 & 82.1 & 85.5 & 92.8 & 75.9 & 94.1 & 80.4 & 65.9 & 100.0 & 99.9 &  70.7 & 61.7 & 91.5 & 84.1 & 83.7  \\
\midrule
% One2Any (Ours) & RGBD  & 4-best view \\
One2Any (Ours) & RGBD  & 8-best view & 85.0 & 93.7 & 97.8 & 84.9 & 94.9 & 90.1 & 73.2 & 100.0 & 99.9 & 88.8 & 89.8 & 95.4 & 85.2 & 90.7\\
One2Any (Ours) & RGBD  & 16-best view & 84.8 & \textbf{98.3} & \textbf{98.8} & \textbf{95.2} & 95.9 & \textbf{93.3} & \textbf{76.2} & \textbf{100.0} & \textbf{99.9} & 92.9 & 95.1 & 94.4 & 93.9 & \textbf{93.8}\\

% FoundPose \cite{wen2024foundationpose} &36.5  &  65.3  & 49.8 & 42.6 & 99.0 & 64.8 & 20.7 & 15.8 & 51.7 & 49.6\\
% NOPE \cite{nguyen2024nope}  & \\
% Oryon \cite{corsetti2024open} & 1.2  & 85.2 & 0.3  & 0.8 & 63.2 & 18.4 & 1.6  &2.9 & 11.7 &   20.6\\
% \midrule
% % Ours & RGBD & \xmark & 1 & 43.4 & 59.3 & 59.7 & 59.3 & 54.4 & 65.7 & 35.8 & 100.0 & 99.9&  55.4 & 28.0 & 52.4 & 53.0 &  \\
% Ours & 33.1  & 66.2  & 68.2 & 35.8 & 100.0 & 99.9&  28.2 & 31.9 & 53.2 & 57.4\\
\bottomrule
\end{tabular}
    \label{tab:multi-view}
\end{table*}

\subsection{Experiments with Multi-view Setups}
We conduct experiments on the challenging LINEMOD dataset \cite{hinterstoisser2011multimodal}, which features significant view variation. Results are presented in Table \ref{tab:multi-view}. In addition, we evaluated the performance of our method with 8 /16  reference views. Using the simple pose selection strategy, our method achieved a 50\% improvement with 8 reference views and a 59\% improvement with 16 reference views. Notably, the performance with 16 reference views surpasses LatentFusion \cite{park2020latentfusion}, which learns an object latent space to render additional views. While FS6D \cite{he2022fs6d} is specifically fine-tuned for the LINEMOD dataset, OnePose \cite{sun2022onepose} and OnePose++ \cite{he2022onepose++} require over 200 reference views to compensate for the lack of depth information but still perform poorly.

However, the simple selection strategy does not always guarantee the optimal predicted pose. To address this, we further analyze the best-case prediction results (last two rows of Table \ref{tab:multi-view}),where the predictions most closely resemble the ground truth. These results show significant improvements, demonstrating that our method outperforms many existing multi-view approaches. 

Furthermore, the experimental results demonstrate that our method has the potential to be further enhanced and explored in multi-view setups, offering even greater capabilities.
